# Supplementary material for: Unified Differentiable Learning of Electric Response
Source: arXiv:2403.17207 source file (2024-06-07)
Supplement: Supplementary file 1 [file SI.pdf]

# Supplementary Information
# Unified Differentiable Learning of Electric Response

Stefano Falletta,[1,*] Andrea Cepellotti,[1] Anders Johansson,[1] Chuin Wei Tan,[1] Albert Musaelian,[1] Cameron J. Owen,[2] and Boris Kozinsky[1,3,†]

[1] *John A. Paulson School of Engineering and Applied Sciences, Harvard University, Cambridge, MA, USA*
[2] *Department of Chemistry and Chemical Biology, Harvard University, Cambridge, MA, USA*
[3] *Robert Bosch LLC Research and Technology Center, Watertown, MA, USA*

## I. COMPUTATIONAL DETAILS

The DFT calculations are performed using a plane-wave density functional approach as implemented in the Quantum Espresso suite [1]. We use the semilocal Perdew-Burke-Ernzerhof (PBE) functional [2], and describe the core-valence interactions using normconserving pseudopotentials [3]. As case studies, we consider $\alpha$-$SiO_2$ and tegragonal $BaTiO_3$. We model $\alpha$-$SiO_2$ with a 72-atom orthorhombic supercell ($a = 9.97$ Å, $b = 8.63$ Å, $c = 10.96$ Å), and $BaTiO_3$ with both 40-atom ($a = 7.97$ Å, $b = 7.97$ Å, $c = 8.45$ Å) and 135-atom ($a = 11.90$ Å, $b = 11.90$ Å, $c = 12.91$ Å) tetragonal supercells. We sample the Brillouin zone with a 2×2×2 k-grid for $\alpha$-$SiO_2$ and for the 40-atom supercell of $BaTiO_3$, and at the $\Gamma$ point for the 135-atom supercell of $BaTiO_3$. The energy cutoff is set to 100 Ry in all cases. The lattice parameters of each system are optimized within these parameters. For the calculation of Born charges and polarizability, the finite electric field is set to $10^{-4}$ Ry a.u. along each Cartesian direction, which ensures a linear regime of polarization with respect to electric field. The DFPT calculations for $\alpha$-$SiO_2$ are performed using a 9-atom supercell and a 4×4×4 kgrid. The infrared spectrum and the frequency-dependent dielectric constant from DFPT are computed at the $\Gamma$-point of the Brillouin zone.

The data frames of $\alpha$-$SiO_2$ are generated through lammps [4], by using the classical Vashishta potential [5]. The time step is set to 2 fs. The data frames of the 135-atom supercell of $BaTiO_3$ are generated through active learning dynamics using the code FLARE [6], interfaced with quantum espresso for DFT calculations and with lammps for MLMD. In particular, we use energy noise of 0.135 eV, force noise of 0.15 eV/Å, stress noise of 0.001 eV/Å$^3$. We employ a B2 ACE descriptor, radial basis of 8, angular basis of 4, and a cutoff radius of 5.0 Å. The active learning dynamics is run in the NVT ensemble with temperature ranging from 300 to 400 K. The time step is set to 2 fs.

The Allegro code is compiled using PyTorch 1.11 [7]. We use 2-layers models with full $O(3)$ symmetry, radial cutoff $r_{\max} = 6$ Å, maximum order of spherical harmonics $\ell_{\max} = 3$, 64 tensor features, and 8 Bessel functions to represent interatomic distances. For both $\alpha$-$SiO_2$ and $BaTiO_3$, the network is constituted of two-body latent multi-layer perceptron (MLP) with hidden dimensions $[64, 64, 64]$, a latent MLP with dimensions $[64, 64, 64]$, a linear projection as embedding MLP, and a single layer of dimension 128 as final MLP. SiLU nonlinearities are applied to the two-body latent MLP and to the latent MLP. We fix the batch size to 1, the learning rate to 0.001, and the scheduler patience to 500. We use the Adam optimizer [8] in PyTorch, with default parameters of $\nu_1 = 0.9$, $\nu_2 = 0.999$, and $\epsilon = 10^{-8}$ without weight decay. For $\alpha$-$SiO_2$, the optimized loss function weights are $\lambda_U = 1$, $\lambda_F = 1$, $\lambda_P = 1$, $\lambda_Z = 10$, and $\lambda_\alpha = 1000$. For $BaTiO_3$, the optimized loss function weights are $\lambda_U = 1$, $\lambda_F = 1$, $\lambda_P = 1$, $\lambda_Z = 1$, and $\lambda_\alpha = 1000$. The dataset is split in 80% for training, and 20% for validation. The validation of our model $\alpha$-$SiO_2$ on the entire dataset yields mean absolute errors of 2.5 meV on per-atom energy, 20.8 meV·Å$^{-1}$ on forces, $9.2 \cdot 10^{-2}$ me·Å on polarization, $5 \cdot 10^{-3}$ on Born charges, and 12 me·A$^2$·V$^{-1}$ on polarizabilities. The validation of our model $BaTiO_3$ on the entire dataset yields mean absolute errors of 0.4 meV on per-atom energy, 12.2 meV·Å$^{-1}$ on forces, 1.1 me·Å on polarization, $13.0 \cdot 10^{-3}$ on Born charges, and 17.9 me·A$^2$·V$^{-1}$ on polarizabilities. Parity plots comparing the DFT labels with the ML predictions are illustrated in Fig. 2. Data distributions of the DFT results are given in Fig. 1.

The lammps code is used for all production relaxations and MD, both in the absence and in the presence of an electric field. The Allegro pair style was extended with methods to extract arbitrary quantities from the output generated by the Allegro PyTorch model. These quantities are then available through an Allegro "compute" for use in output and analysis, which in this project was used to extract the polarization and polarizability. For performing dynamics under an electric field, we developed a "fix" for adding the extra contribution to the energy, forces, and polarization. The implementation is modeled after the existing "fix addforce" and allows for time- and space-dependent electric fields applied to a subset of the atoms. For atomic relaxations we use the minimization style denoted 'fire' [9].

* stefanofalletta@g.harvard.edu
† bkoz@g.harvard.edu

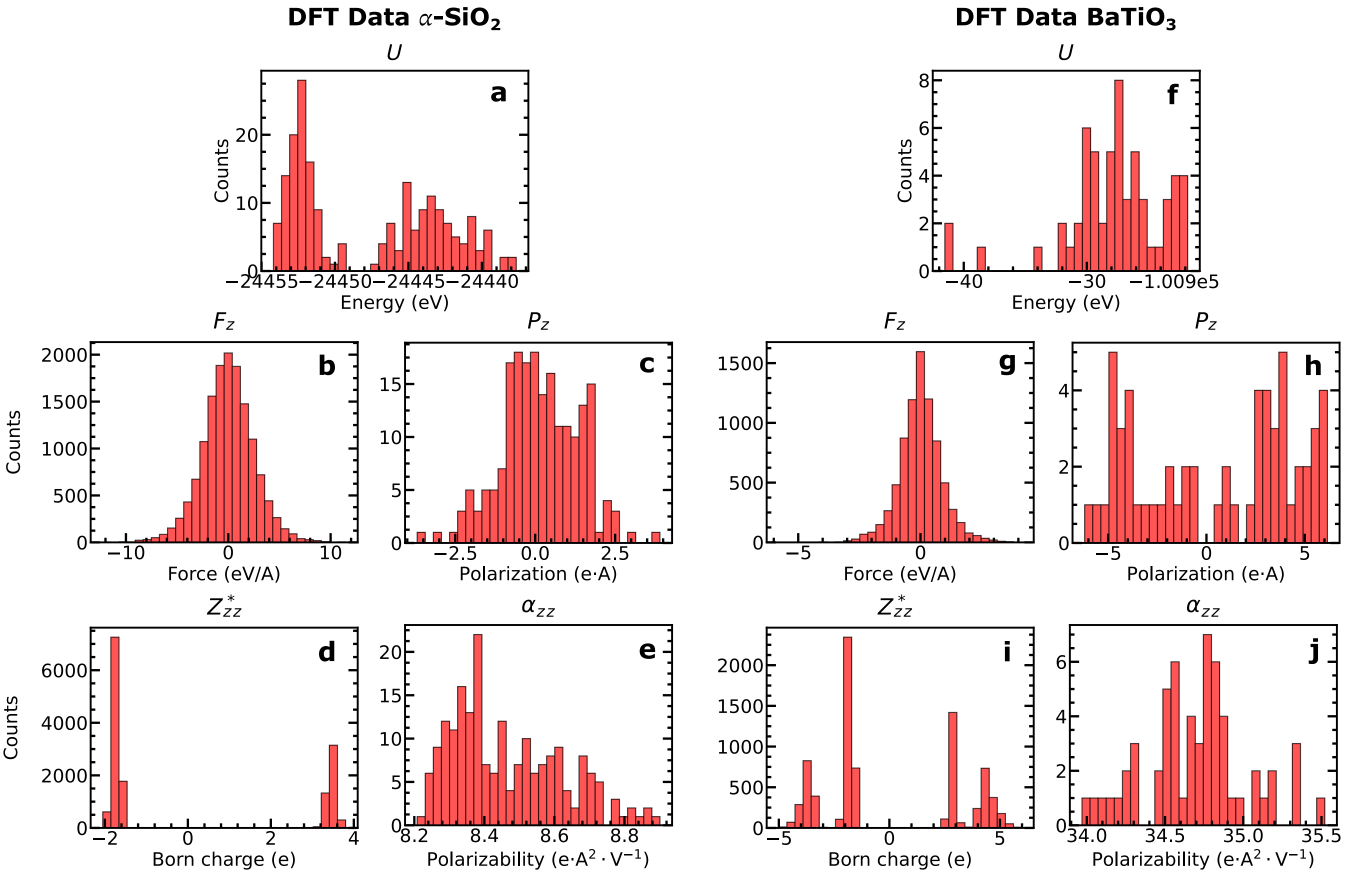


FIG. 1. **DFT Data of $\alpha$-SiO$_2$ and BaTiO$_3$**. Histograms of energy, forces, polarization, Born charges, and polarizability obtained with DFT and with our unified ML model. Each $\mu$ component of polarization is folded in the range $[-\frac{1}{2}\Delta P_\mu, +\frac{1}{2}\Delta P_\mu]$, where $\Delta\mathbf{P}$ is the quantum of polarization. All quantities are determined in the limit of vanishing electric field.

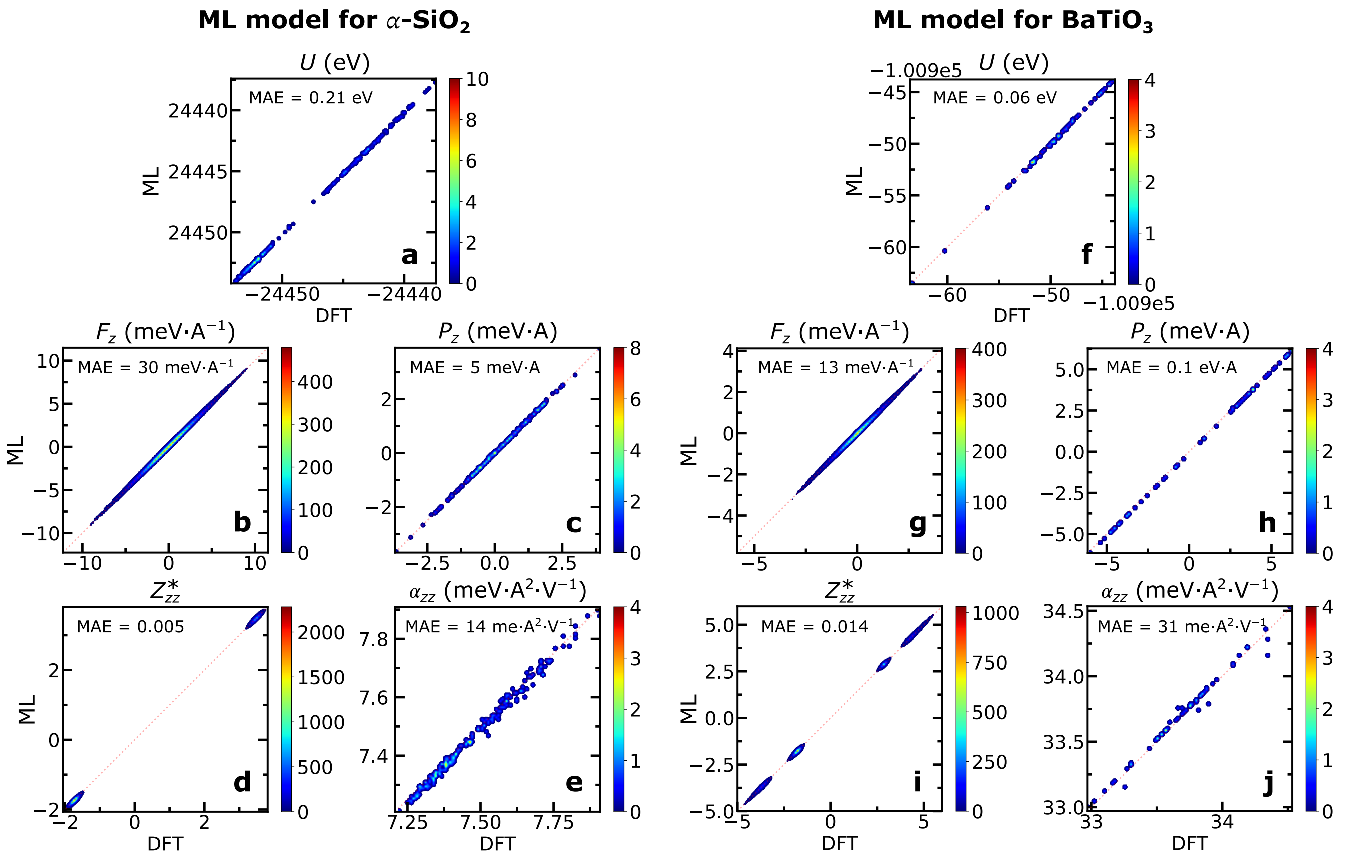


FIG. 2. **Accuracy of the ML models for $\alpha$-$SiO_2$ and $BaTiO_3$.** Parity plots of energy, forces, polarization, Born charges, and polarizability comparing the results obtained with DFT and with our unified ML model. Each $\mu$ component of polarization is folded in the range $[-\frac{1}{2}\Delta P_\mu, +\frac{1}{2}\Delta P_\mu]$, where $\Delta \mathbf{P}$ is the quantum of polarization. Mean absolute errors (MAE) are provided in the inset of the plots. All quantities are determined in the limit of vanishing electric field.


[1] P. Giannozzi, S. Baroni, N. Bonini, M. Calandra, R. Car, C. Cavazzoni, D. Ceresoli, G. L. Chiarotti, M. Cococcioni, I. Dabo, A. D. Corso, S. de Gironcoli, S. Fabris, G. Fratesi, R. Gebauer, U. Gerstmann, C. Gougoussis, A. Kokalj, M. Lazzeri, L. Martin-Samos, N. Marzari, F. Mauri, R. Mazzarello, S. Paolini, A. Pasquarello, L. Paulatto, C. Sbraccia, S. Scandolo, G. Sclauzero, A. P. Seitsonen, A. Smogunov, P. Umari, and R. M. Wentzcovitch, QUANTUM ESPRESSO: a modular and open-source software project for quantum simulations of materials, J. Phys.: Condens. Matter **21**, 395502 (2009).

[2] J. P. Perdew, K. Burke, and M. Ernzerhof, Generalized gradient approximation made simple, Phys. Rev. Lett. **77**, 3865 (1996).

[3] M. van Setten, M. Giantomassi, E. Bousquet, M. Verstraete, D. Hamann, X. Gonze, and G.-M. Rignanese, The PseudoDojo: Training and grading a 85 element optimized norm-conserving pseudopotential table, Comput. Phys. Commun. **226**, 39 (2018).

[4] S. Plimpton, Fast parallel algorithms for short-range molecular dynamics, J. Comput. Phys. **117**, 1 (1995).

[5] J. Q. Broughton, C. A. Meli, P. Vashishta, and R. K. Kalia, Direct atomistic simulation of quartz crystal oscillators: Bulk properties and nanoscale devices, Phys. Rev. B **56**, 611 (1997).

[6] J. Vandermause, S. B. Torrisi, S. Batzner, Y. Xie, L. Sun, A. M. Kolpak, and B. Kozinsky, On-the-fly active learning of interpretable bayesian force fields for atomistic rare events, npj Comput. Mater. **6**, 20 (2020).

[7] A. Paszke, S. Gross, F. Massa, A. Lerer, J. Bradbury, G. Chanan, T. Killeen, Z. Lin, N. Gimelshein, L. Antiga, A. Desmaison, A. Kopf, E. Yang, Z. DeVito, M. Raison, A. Tejani, S. Chilamkurthy, B. Steiner, L. Fang, J. Bai, and S. Chintala, PyTorch: An imperative style, high-performance deep learning library, in *Adv. Neural Inf. Process. Syst.*, Vol. 32, edited by H. Wallach, H. Larochelle, A. Beygelzimer, F. d'Alché-Buc, E. Fox, and R. Garnett (Curran Associates, Inc., 2019).

[8] D. P. Kingma and J. Ba, Adam: A method for stochastic optimization (2017), arXiv:1412.6980.

[9] E. Bitzek, P. Koskinen, F. Gähler, M. Moseler, and P. Gumbsch, Structural relaxation made simple, Phys. Rev. Lett. **97**, 170201 (2006).
